# Supplementary material for: FlowBack-Adjoint: Physics-Aware and Energy-Guided Conditional Flow-Matching for All-Atom Protein Backmapping
Source: arXiv:2508.03619 ancillary file (2025-08-05)
Supplement: Supplementary file 1 [file supplementary.pdf]

# SUPPORTING INFORMATION
# FLOWBACK-ADJOINT: PHYSICS-AWARE AND ENERGY-GUIDED CONDITIONAL FLOW-MATCHING FOR ALL-ATOM PROTEIN BACKMAPPING

A PREPRINT

**Alex Berlaga**
Department of Chemistry
University of Chicago, Chicago, IL 60615, USA
berlaga@uchicago.edu

**Michael S. Jones**
Lawrence Livermore National Laboratory, Livermore, CA 94550, USA
jones313@llnl.gov

**Andrew L. Ferguson**
Pritzker School of Molecular Engineering
University of Chicago, Chicago, IL 60615, USA
andrewferguson@uchicago.edu

## A.1 Model Parameters

### A.1.1 Chirality, Lennard-Jones, and Bonded Auxiliary Velocities in FLOWBACK+LJ/BONDS

To transform coarse side-chain coordinates into clash-free, force-field-compatible structures we employ a lightweight Euler integrator. Coordinates are advanced along a schedule $t_0 = 0 \to t_N = 1$ with uniform step $\Delta t = 1/N$,

$$x_{k+1} = x_k + v_\theta(x_k, t_k)\Delta t,$$

where the drift,

$$v_\theta = v_\gamma(x_k, t_k) + \mathbf{1}_{t_k \geq 0.25}\, v_{\text{chiral}} + \mathbf{1}_{t_k \geq 0.85}\, \frac{t_k^\alpha}{10}\, v_{\text{LJ}} + \mathbf{1}_{t_k \geq 0.95}\, t_k^\alpha\, v_{\text{bond}},$$

combines augments the learned, unmasked EGNN velocity field $v_\gamma(x_k, t_k)$ from FLOWBACK, with three auxiliary time-gated velocity fields that adjust the chirality, Lennard-Jones (LJ) interactions, and bond lengths. $\mathbf{1}_{t \geq \tau}$ denotes an indicator function that is zero for $t < \tau$ and unity for $t \geq \tau$. The scaling of the LennardJones (L-J) velocities by $\frac{t_k^\alpha}{10}$ and the bonded velocities by $t_k^\alpha$ is intended as a heuristic annealing schedule: at early integration steps, the scale factors are tiny, so both non-bonded and bonded forces are almost zero. As the trajectory advances and $t_k \to 1$, the factors grow rapidly with scaling $t_k^\alpha$, progressively switching on the full force constants when the atoms become close to their physically realistic geometry. Empirically, we find an exponent of $\alpha = 20$ together with the $\frac{1}{10}$ pre-factor on the LJ term to perform well in practice.

**Chirality.** In place of FLOWBACK's original discrete side-chain flipping protocol, we inject a continuous, differentiable velocity field $v_{\text{chiral}}$ for $t \geq 0.25$ that smoothly steers any D-form residue toward the correct L-form configuration thereby enforcing native stereochemistry without breaking gradient flow. For a residue with atoms $(\mathrm{N}, \mathrm{C}_\alpha, \mathrm{C}, \mathrm{C}_\beta)$ we monitor the volume,

$$V = \big(N - C_\alpha\big) \times \big(C - C_\alpha\big) \;\cdot\; \big(C_\beta - C_\alpha\big),$$

where a positive volume implies a desirable L-chirality, whereas a negative volume implies an undesirable D-chirality. For each Euler step we compute a target increment for each amino acid residue, $\Delta V$,

$$\Delta V = \begin{cases} \varepsilon - V, & V < 0 \quad \texttt{(FLIP)}, \\ V_{\text{ref}}(t) - V, & 0 \leq V < V_{\text{ref}}(t) \quad \texttt{(PUSH)}, \\ 0, & \text{otherwise}, \end{cases}$$

where FLIP is a velocity that reflects the side chain across the symmetry plane, PUSH is a velocity that guides the residue from an aphysical position on or near the reflection plane to its expected positive-volume positions relative to the reflection plane, $V_{\text{ref}}(t)$ = $2{\times}10^{-3}t^3$ nm$^3$ acts as a cutoff set to about 80-90% of, yet always below, the volume expected at integration time $t$, and $\varepsilon = 2{\times}10^{-4}$ nm$^3$ prevents instabilities in normalizing the velocity vectors. This increment is then converted into a velocity as follows. First, to determine the magnitude of the velocity on every atom, we compute,

$$k_{\text{side}} = \texttt{clip}\left(\frac{\Delta V}{A\,\Delta t},\ 0,\ k_{\max}\right),$$

where $A = \big\|(N - C_\alpha) \times (C - C_\alpha)\big\|$ is the area of the parallelogram spanned by these three backbone atoms – and hence, $k_{\text{side}}$ increases in proportion to the magnitude of the chirality error component normal to the reflection plane – and the clipping operation delimits the outputted value to the range $[0, k_{\max}]$, where $k_{\max}$ = 1.2 nm/timestep. We then compute the direction of the chriality velocity by projecting the normal vector of the chirality reflection plane onto the plane normal to the $\mathrm{C}_\alpha$–$\mathrm{C}_\beta$ bond to keep that bond length stable,

$$\hat{n}_\perp = \hat{n} - (\hat{n}\cdot u_\beta)\, u_\beta, \quad \text{where} \quad u_\beta = \frac{C_\beta - C_\alpha}{\|C_\beta - C_\alpha\|} \quad \text{and} \quad \hat{n} = ((N - C_\alpha) \times (C - C_\alpha))/A.$$

However, not all atoms are applied a uniform velocity: we note that the backbone N, $\mathrm{C}_\alpha$, and C are not affected by this operation, as they define the chirality reflection plane. All remaining atoms in the residue are subject to velocities,

$$v_{\text{chiral}} = \begin{cases} +k_{\text{side}}\, \hat{n}_\perp & \text{for side-chain atoms} \\ -\frac{1}{2} k_{\text{side}}\, \hat{n}_\perp & \text{for the backbone oxygen}, \end{cases}$$

with the backbone O atom velocity scaled by 50% to avoid backbone distortions and instability due to overcorrection.

**Lennard-Jones.** A Lennard-Jones (LJ) velocity term $v_{\text{LJ}}$ is introduced for $t \geq 0.85$, wherein close-range heavy-atom pairs are subjected to a Lennard-Jones interaction under the CHARMM27 molecular mechanics force field [MacKerell Jr. et al., 2000]. Specifically, for each protein heavy-atom pair $(i, j)$ topologically separated by more than two covalent bonds and possessing an inter-atomic distance $r_{ij} = \|x_i - x_j\| < 0.42$ nm, we compute the Lennard-Jones force,

$$F_{ij} = 24\frac{\epsilon_{ij}}{r_{ij}^2}\left[2\left(\frac{\sigma_{ij}}{r_{ij}}\right)^{12} - \left(\frac{\sigma_{ij}}{r_{ij}}\right)^{6}\right](x_i - x_j),$$

where $\sigma_{ij} = (\sigma_i + \sigma_j)/2$ and $\epsilon_{ij} = \sqrt{\epsilon_i \epsilon_j}$ for chemically dissimilar atom types are computed as prescribed by the Lorentz-Berthelot mixing rules [Lorentz, 1881, Berthelot, 1898, Lennard-Jones, 1929, Allen and Tildesley, 2017].

The Lennard-Jones force on atom $i$ is converted into a corresponding velocity correction for atom $i$ by summing over all pairwise interactions to resolve the net force $F_i$ experienced by atom $i$, dividing by the mass of atom $i$ to compute the net acceleration $a_i = F_i/m_i$, and then multiplying by a single time step,

$$v_{\text{LJ}_i} = \frac{\Delta t}{m_i}\sum_{j \neq i} F_{ij}.$$

The additional velocity introduced by this auxiliary force is capped at a magnitude of $v_{LJ}$ = 5 nm/timestep to preserve stability of the Euler integrator.

**Bonds.** For ($t \geq 0.95$), a harmonic bond length interaction is added around the equilibrium bond length mandated by the CHARMM27 molecular mechanics force field MacKerell Jr. et al. [2000]. For each bonded pair $(i, j)$ with ideal bond length $b_0$ and spring constant $k_b$ we evaluate the bonded force,

$$F_{ij}^{\text{bond}} = k_b\big(r_{ij} - b_0 t\big)(x_i - x_j),$$

and compute the corresponding velocity update as,

$$v_{\text{bond}_i} = -\frac{\Delta t}{m_i}F_{ij}^{\text{bond}}, \qquad v_{\text{bond}_j} = +\frac{\Delta t}{m_j}F_{ij}^{\text{bond}}.$$

The additional velocity introduced by this auxiliary force is capped at a magnitude of $v_{bond}$ = 1 nm/timestep to preserve stability of the Euler integrator.

### A.1.2 FLOWBACK Training Parameters

All calculations were performed on a single NVIDIA L40S GPU, which enabled efficient evaluation of the vector field over large molecular graphs using tensor cores. Training was conducted with a batch size of one protein, and the Gaussian noise added to the interpolated structure was fixed at $\sigma_{int} = 0.005$ nm. The prior noise applied to coarse-grained inputs was $\sigma_p = 0.003$ nm. The EGNN was trained to learn a vector field $v(x, t, M)$ by regressing against the reference field $u_t = (x_1 - x_0)$ under an $L1$ loss. Operationally, we "trick" the EGNN into learning the drift $v_\gamma(x_t, t, M)$ by training it to predict a one-step-ahead configuration $x_t' = EGNN_\gamma(x_t, t, M)$ and then computing $v_\gamma(x_t, t, M) = (x_t' - x_t)$. Training is conducted for 15 epochs using the Adam optimizer [Kingma and Ba, 2014] with a learning rate of 0.001. The model architecture consists of a six-layer $E(3)$-equivariant graph neural network [Batzner et al., 2022, Liao and Smidt, 2022], with message passing between each node and its 15 nearest neighbors. The latent-space dimension of was 32. Both node and message embeddings were passed with `SiLU` nonlinearity. Vector field updates were clamped to a maximum magnitude of 2 nm/timestep.

### A.1.3 FLOWBACK-ADJOINT Training Parameters

Adjoint matching was performed over all-atom trajectories of nine fast-folding mini-proteins in water conducted by D.E. Shaw Research (DESRES) [Lindorff-Larsen et al., 2011]:

1. BBA - 28-residue $\beta\beta\alpha$ miniprotein (PDB ID: `1FME`)
2. BBL - 47 residue ultrafast protein folder (PDB ID: `2WXC`)
3. $\lambda$-repressor fragment - 80-residue switch protein fragment (PDB ID: `1LMB`)
4. NTL9 - 39-residue N-terminal domain of ribosomal protein L9 (K12M mutation, PDB ID: `2HBA`)
5. Chignolin - 10-residue synthetic mini-protein (PDB ID: `1UAO`)
6. Trp-cage (TC5b) - 20-residue $\alpha/\pi$ miniprotein (PDB ID: `2JOF`)

7. Protein G - 56-residue fast-folding GB1 variant (PDB ID: 1IGD)
8. UVF - 52-residue homeodomain variant (PDB ID: 2P6J)
9. $\alpha$3D - 73-residue de novo three-helix bundle (PDB ID: 2A3D).

For each trajectory frame, we generated one output sample using an Euler integrator with 100 integration steps through the reference trajectory. Weights were loaded from the pre-trained FLOWBACK model. The coarse-grained prior noise was fixed at 0.003 nm. The adjoint matching objective was optimized using the Adam optimizer with a learning rate of $10^{-5}$. Gradient accumulation was used across 16 mini-batches and energy gradients were clipped at a a maximum gradient norm of 20 nm/timestep. In the selection of $\mathcal{T}$ during the computation of the adjoint matching loss, using a similar protocol to Domingo-Enrich et al. [2025], we included all timesteps $t > 0.8$, as well as 10 values of $t \leq 0.8$ selected form a uniform distribution. The regularization parameter for the adjoint loss was set to $\lambda = 0.01$, and the CHARMM27 molecular mechanics force field MacKerell Jr. et al. [2000] used to evaluate energies and forces. We scaled GPU memory usage to 24 GB to fit within hardware constraints by controlling the accumulating batch size during the calculation of $\mathcal{L}_{\text{adjoint}}$.

## A.2 Simulation Parameters for Molecular Dynamics Stability Test

All-atom MD simulations of the backmapped configurations are initialized by generating from each heavy-atom structure a CHARMM27 topology file using `gmx pdb2gmx` to place hydrogens and employing pH 7 protonation states. The resulting files are converted into an OpenMM simulation input file [Eastman et al., 2017]. The cubic unit cell is padded by 2 nm in each dimension. Electrostatics are evaluated using Particle Mesh Ewald (PME) with a 1.0 nm real-space cutoff. Dynamics are propagated in the canonical (NVT) ensemble at $T = 300$ K using a Langevin integrator with collision frequency $\gamma = 1$ ps$^{-1}$ and time-step 1 fs. All covalent bonds involving hydrogens are constrained and center-of-mass motion is removed every 1 ps. A 100-step pre-run is used to detect immediate pathologies in the initialization (e.g., NaN positions or energies). Upon passing this pre-check, the simulation is continued for 20,000 time steps (20 ps). A trajectory is deemed stable when (i) the simulation finishes without exception, (ii) no NaNs appear in energies or coordinates, and (iii) the largest Cartesian force on any heavy atom during the pre-check remains finite. These simulations are very inexpensive and typically complete in <10 s on a single NVIDIA V100 GPU.

To assess the influence of hydrogen-atom placement on the stability of the MD simulation, we also conducted calculations in which the hydrogen atoms and termini were deleted, their partial charges to their neighboring atoms, and simulations conducted treating these groups as united atoms that experience exactly the same bonded forces as their original forms. In this case, the absence of hydrogen atoms permitted us to employ a larger 2 fs time step and conduct 20,000 time steps (40 ps) simulations. All other simulation parameters remained the same.

## A.3 BLAST

We confirmed via a BLAST search that none of these proteins shared more than 60% identity with any entry in the SidechainNet training corpus [King and Koes, 2021] that was used to train the original FLOWBACK model or any of the nine DESRES proteins [Lindorff-Larsen et al., 2011] used to train FLOWBACK-ADJOINT, thereby guarding against any observed improvements over this test set resulting from data leakage or high sequence similarity with sequences in the training set.

1. **Database construction.** All SidechainNet chains were exported to a single FASTA file with the SidechainNet Python API (v1.0.1) and converted into a local protein database using BLAST+ (v2.15.0) [Camacho et al., 2009]. The same process was applied to the 9 DESRES training proteins.
2. **Query preparation.** The primary sequence of each OOD60 test chain was written to an individual FASTA file, preserving its PDB chain identifier.
3. **BLAST search.** Each query was aligned against the SidechainNet database with default composition-based statistics, soft segmentation, an *E*-value cutoff of $10^{-3}$, and retrieval of up to 5000 target sequences.
4. **Filtering criteria.** Alignments were retained only if they satisfied all of the following: (i) alignment length greater than 70 % of the query chain, (ii) percentage identity $\geq 30\,\%$, and (iii) *E*-value $\leq 10^{-3}$. For each query we recorded the maximum percentage identity observed across all remaining hits.
5. **Sequence identity threshold.** A protein was included in our OOD60 test set only if its best SidechainNet hit exhibited $< 60\,\%$ sequence identity.

## A.4 Supplementary Figures

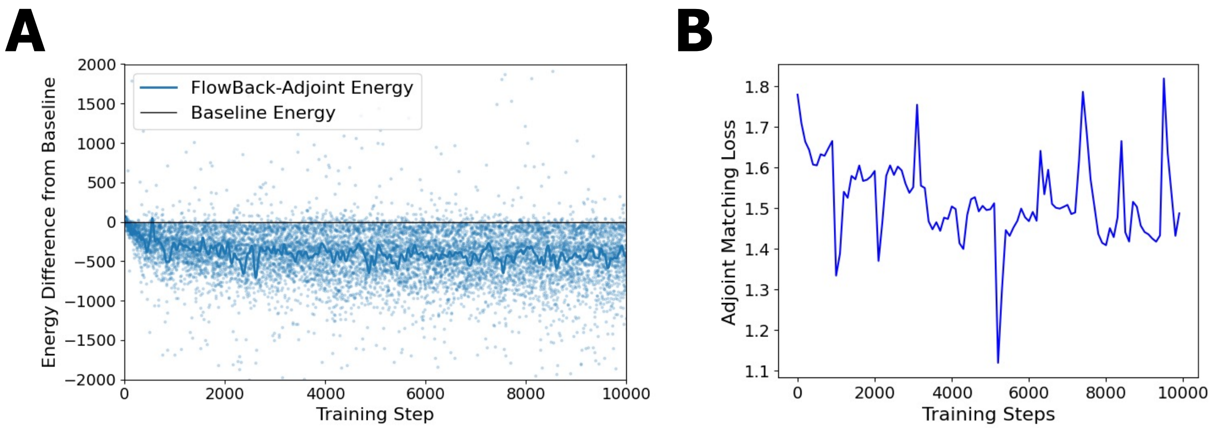


Figure A.1: Fine-tuning of FLOWBACK-ADJOINT. (A) Plot of the FLOWBACK-ADJOINT CHARMM27 potential energy relative to the FLOWBACK+LJ/BONDS baseline. The difference is plotted as blue points and the dark blue line represents a smoothed average using a Gaussian kernel. (B) The average adjoint matching loss recorded at 100 training step intervals. Several checkpoints are taken for validation against the WW Domain and Protein B. The checkpoint at step 7000 is used as the final model.

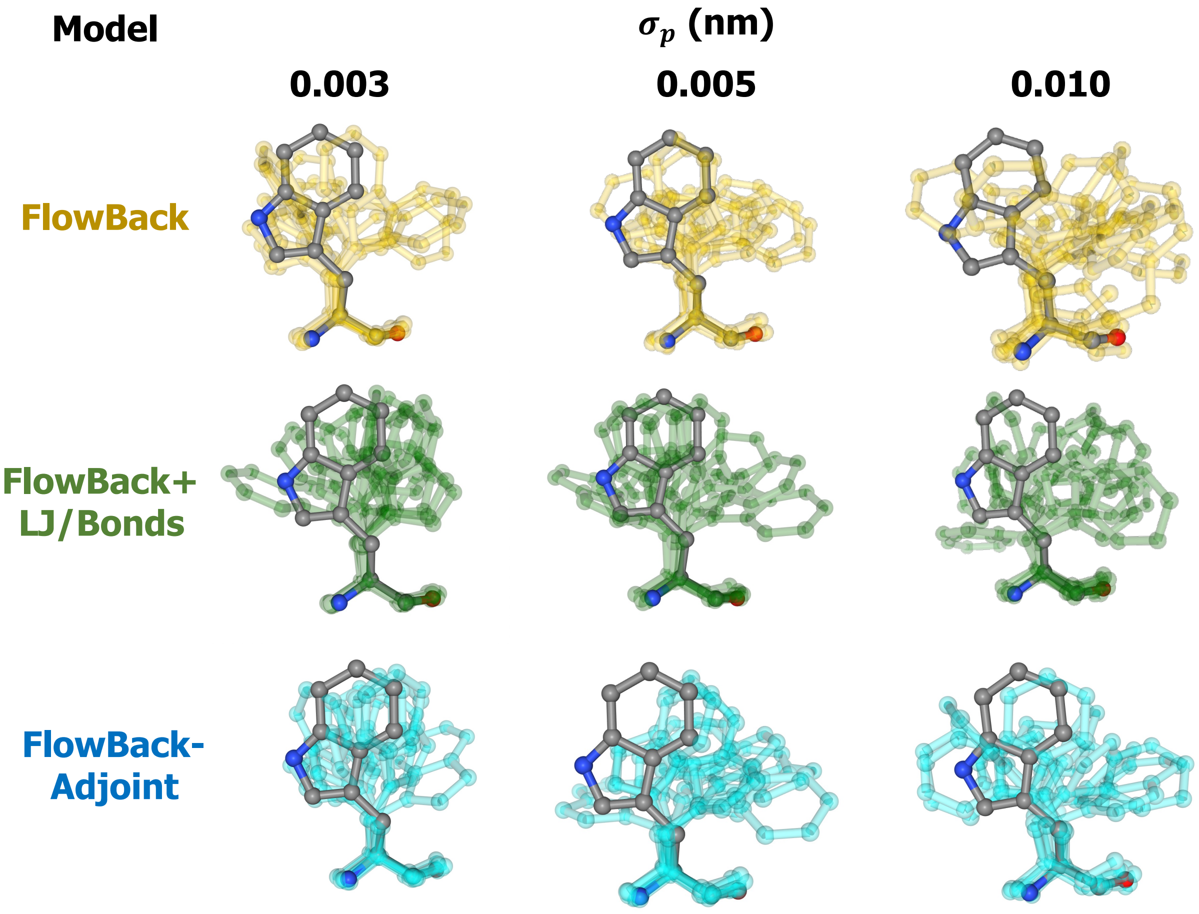


Figure A.2: Visualization of ensembles of 10 AA reconstructions produced by FLOWBACK, FLOWBACK+LJ/BONDS, and FLOWBACK-ADJOINT at choices of the prior noise $\sigma_p$ = 0.003 nm, 0.005 nm, and 0.010 nm around the Trp8 residue of Protein B. Higher values of $\sigma_p$ produce more diverse structural ensembles, but whereas this results in a significant degradation of the structural accuracy of the configurations produced by FLOWBACK and FLOWBACK+LJ/BONDS – including distortions in the aromatic tryptophan rings and other unrealistic elements of the chemical structure – FLOWBACK-ADJOINT breaks this trade-off and can achieve high diversity ensembles that maintain high structural accuracy in terms of bond and clash scores even at high noise values (cf. Table 1).

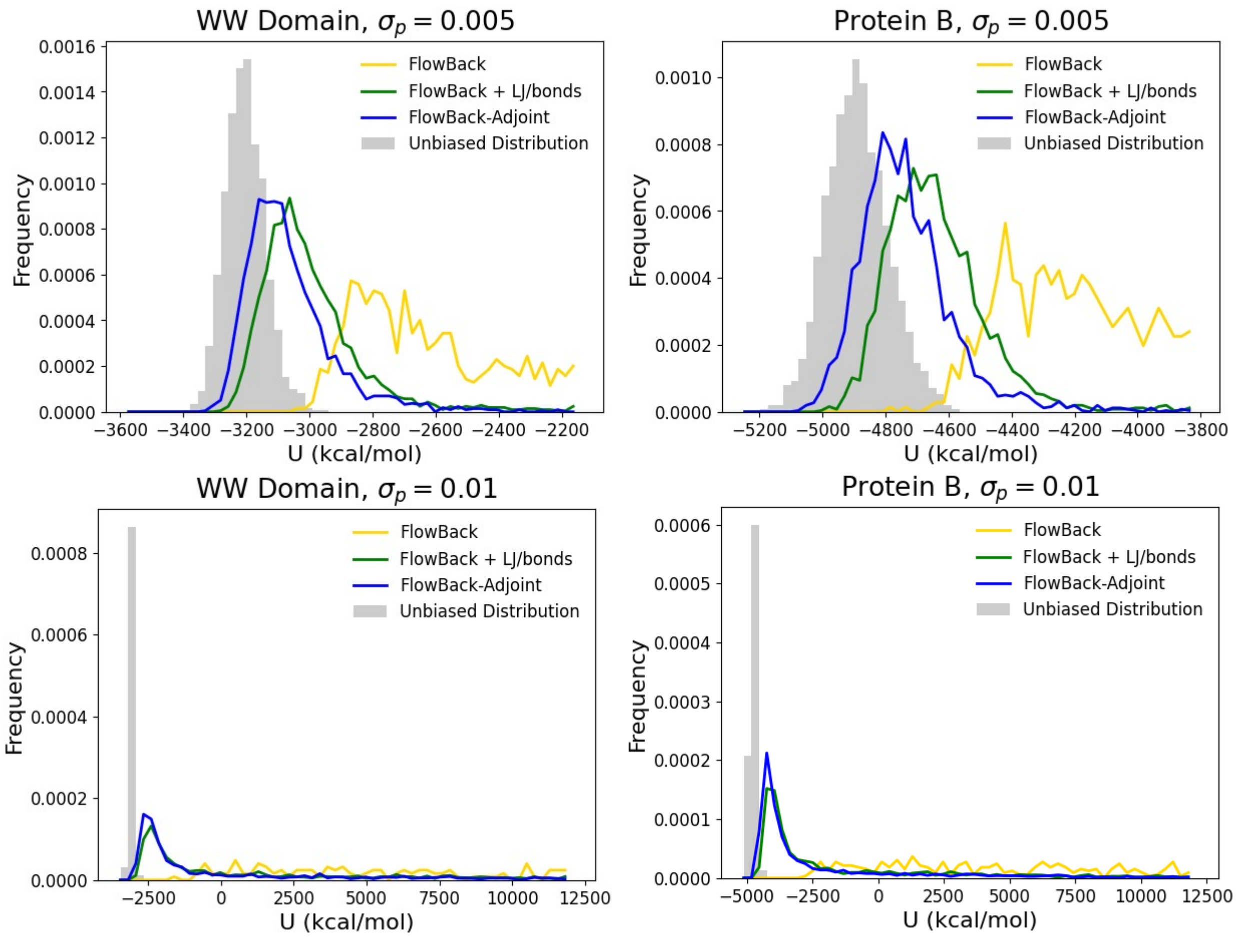


Figure A.3: Distribution of potential energies over an ensemble of 2230 (WW domain) or 2602 (Protein B) backmapped AA configurations from FLOWBACK (yellow), FLOWBACK+LJ/BONDS (green), and FLOWBACK-ADJOINT (blue) at noise values of $\sigma_p = 0.003$ nm (top row) and 0.010 nm (bottom row) for the two hold-out DESRES trajectories of WW domain (left column) and Protein B (right column) [Lindorff-Larsen et al., 2011].

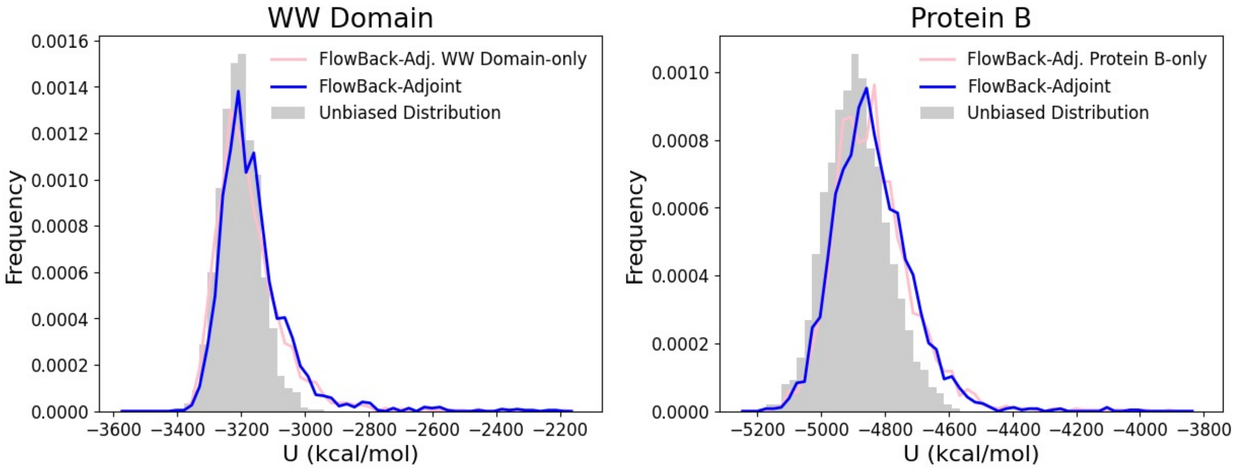


Figure A.4: Distributions of potential energies over an ensemble of 2230 AA configurations of the WW domain and 2602 configurations of Protein B generated by FLOWBACK-ADJOINT at a noise level of $\sigma_p = 0.003$ nm. The blue distribution corresponds to that generated by the general FLOWBACK-ADJOINT model trained over nine DESRES protein trajectories, which did not include WW domain or Protein B, such that the predictions therefore represent an out-of-sample test. The pink distribution corresponds to that generated by the FLOWBACK-ADJOINT model trained on either WW domain or Protein B and then used to generate in-sample predictions. The gray distribution represents the energy distribution over the DESRES MD simulation trajectories of WW domain and Protein B.

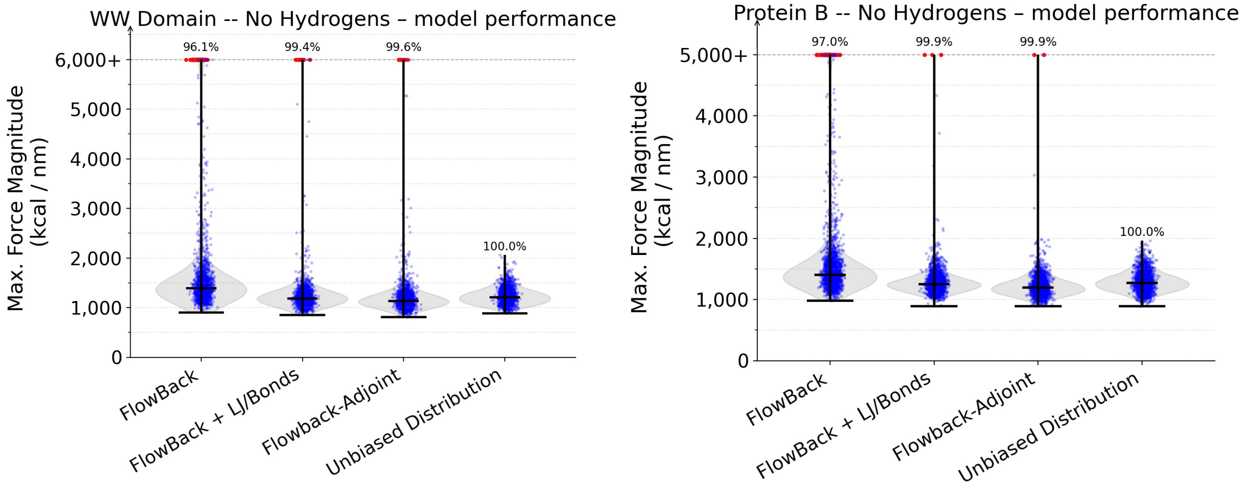


Figure A.5: Swarm and violin plots of the distribution of the maximum force magnitudes experienced by any atom in over the course of a 40 ps MD simulation initialized from a backmapped AA configuration using FLOWBACK, FLOWBACK+LJ/BONDS, FLOWBACK-ADJOINT, or harvested from the MD simulation trajectory. All models employ a noise level of $\sigma_p = 0.003$ nm. In this analysis, hydrogen atoms and termini were deleted, their partial charges to their neighboring atoms, and simulations conducted treating these groups as united atoms that experience the same bonded forces as their original forms. Statistics for each model are aggregated over 2230 (WW domain) or 2602 (Protein B) initial AA configurations and the maximum force identified on any atom in first frame of the molecular-dynamics simulation (i.e. the model-generated structure). For clarity of exposition, large forces in excess of 6,000 kcal/nm are collapsed together at the top of the plot. Test runs in which the MD simulation remained stable over the course of the 40 ps run (i.e. the simulation doesn't crash due to energy, position, or velocity values exceeding floating point limits) have their corresponding points in the swarm colored blue and those which destabilized are colored red. The lowest and median maximum atom-wise force in each swarm plot are indicated by horizontal lines and the overall success rate of stable MD simulation runs is noted as a percentage at the top of each violin.

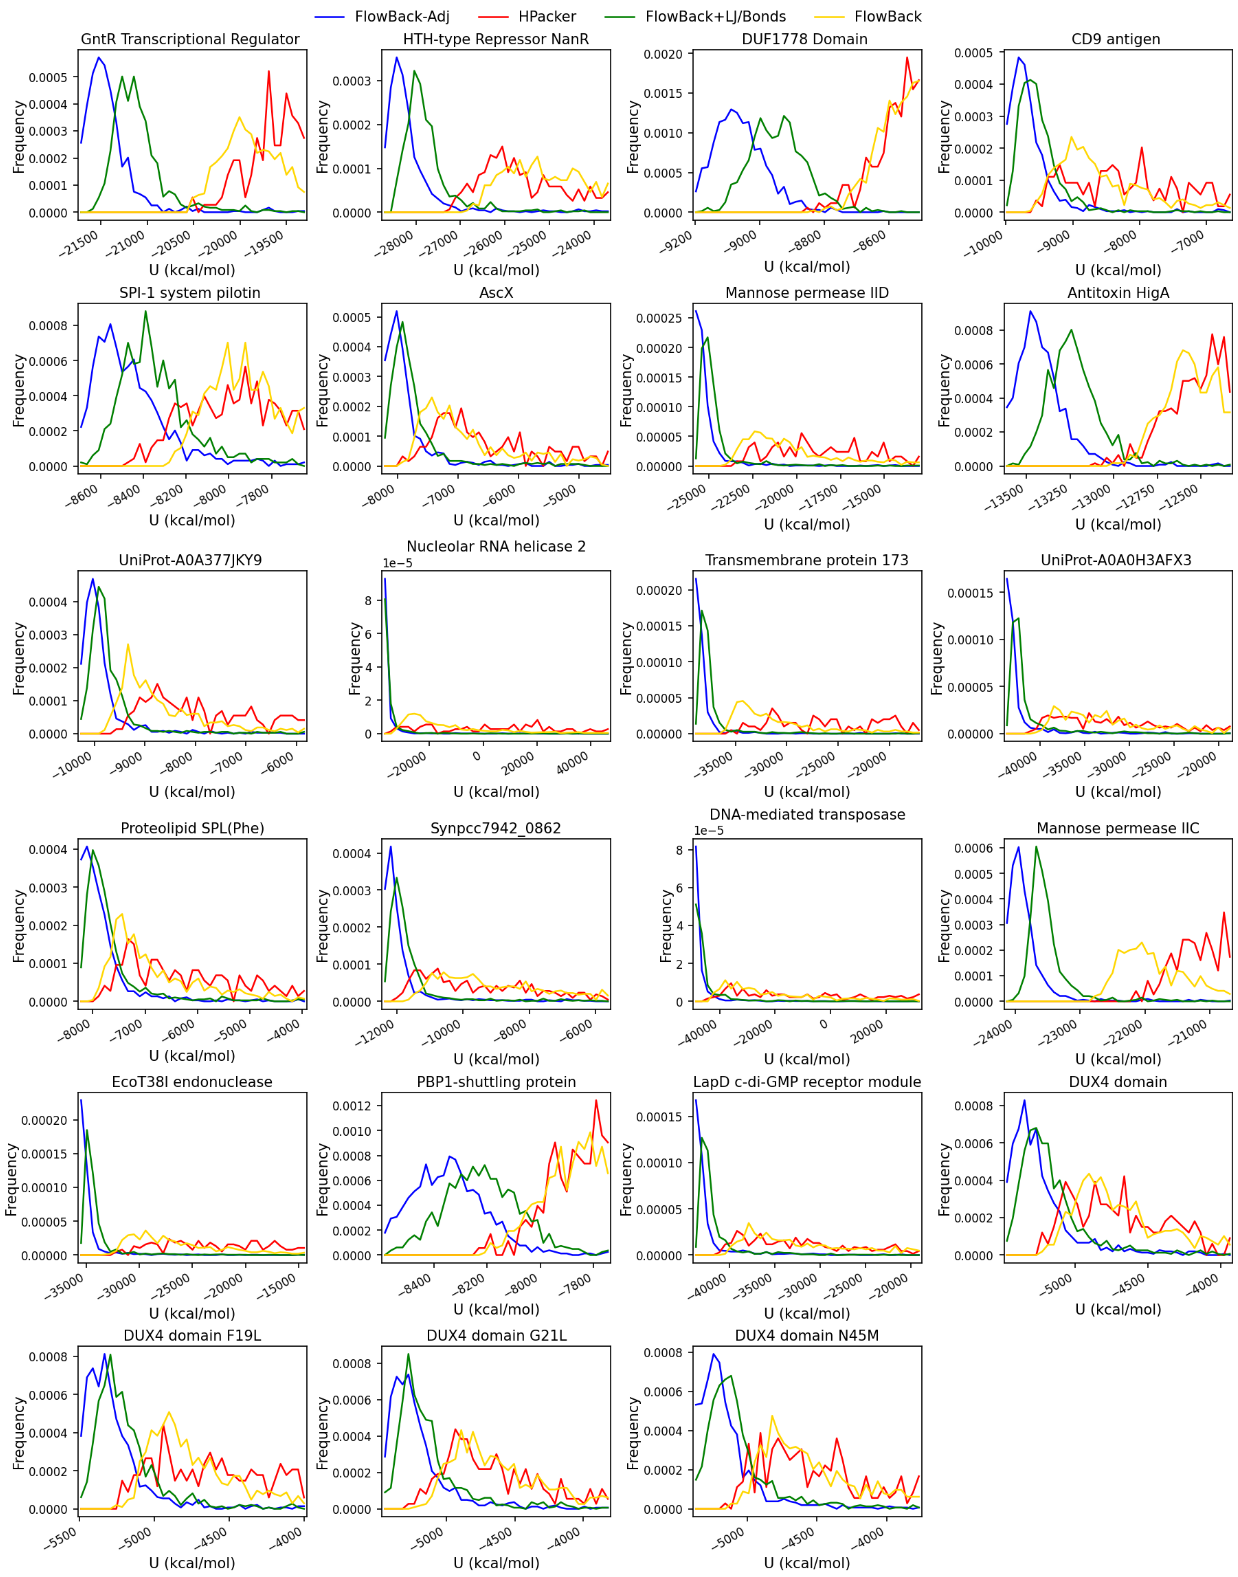


Figure A.6: Potential energy distributions for the AA configurations generated by FLOWBACK-ADJOINT, FLOWBACK+LJ/BONDS, FLOWBACK, and HPACKER from 1000 backbone-only BIOEMU structures generated for the 23 test proteins. In all cases, FLOWBACK-ADJOINT produces lower-energy (i.e., more stable) distributions.

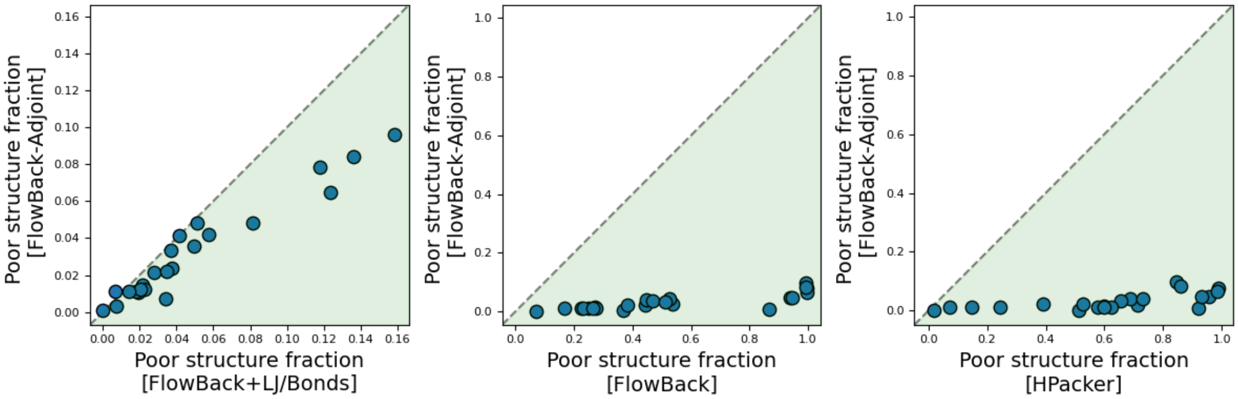


Figure A.7: Fractions of "poor structures" in each of the proteins in our out-of-distribution test. A "poor structure" is defined as one with an energy over 10,000 kcal/mol higher than the median FLOWBACK-ADOINT energy for a given protein, indicating a serious distortion in one or more of the backmapped residues. FLOWBACK-ADJOINT produced fewer poor structures than any other model for any protein, except for 3/23 proteins for which FLOWBACK+LJ/BONDS produced an equal number or fewer poor structures than FLOWBACK-ADJOINT. Both FLOWBACK and HPACKER have several proteins for which more than half of the structures are deemed poor.

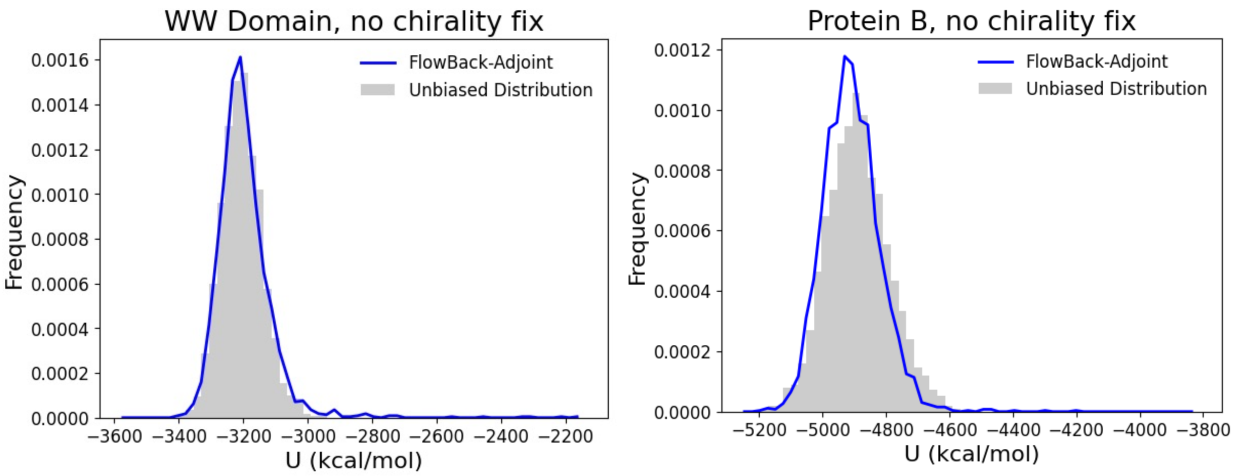


Figure A.8: Distributions of potential energies over an ensemble of 2230 AA configurations of the WW domain and 2602 configurations of Protein B generated FLOWBACK-ADJOINT at a noise level of $\sigma_p$ = 0.003 nm in the absence of the chirality correction. The blue distribution corresponds to that generated by the general FLOWBACK-ADJOINT model trained over nine DESRES protein trajectories, which did not include WW domain or Protein B, such that the predictions therefore represent an out-of-sample test. The gray distribution represents the energy distribution over the DESRES MD simulation trajectories of WW domain and Protein B. Eliminating the chirality correction results in 1-3% of residues with the incorrect D-form chirality, but the energy distributions show far better agreement than when this correction is active with KL divergences falling from 0.0018 $\rightarrow$ 0.0004 for WW domain and 0.0017 $\rightarrow$ 0.0004 for Protein B, indicating almost perfect matching.

## References

Alexander D. MacKerell Jr., Nilesh Banavali, and Nicolas Foloppe. Development and current status of the CHARMM force field for nucleic acids. *Biopolymers*, 56(4):257–265, 2000.

Hendrik Antoon Lorentz. Ueber die anwendung des satzes vom virial in der kinetischen theorie der gase. *Annalen der Physik*, 248(1):127–136, 1881.

D. Berthelot. Sur le mélange des gaz. *Comptes Rendus Hebdomadaires des Séances de l'Académie des Sciences*, 126: 1703–1706, 1898.

J. E. Lennard-Jones. The electronic structure of some diatomic molecules. *Transactions of the Faraday Society*, 25: 668–686, 1929.

Michael P Allen and Dominic J Tildesley. *Computer Simulation of Liquids*. Oxford University Press, 2nd edition, 2017.

Diederik P Kingma and Jimmy Ba. Adam: A method for stochastic optimization. *arXiv preprint arXiv:1412.6980*, 2014.

Simon Batzner, Albert Musaelian, Lixin Sun, Mario Geiger, Jonathan P Mailoa, Mordechai Kornbluth, Nicola Molinari, Tess E Smidt, and Boris Kozinsky. E(3)-equivariant graph neural networks for data-efficient and accurate interatomic potentials. *Nature Communications*, 13(1):2453, 2022.

Yi Liao and Tess E. Smidt. Equiformer: Equivariant graph attention transformer for 3D atomistic graphs. *arXiv preprint arXiv:2206.11990*, 2022.

Kresten Lindorff-Larsen, Stefano Piana, Ron O. Dror, and David E. Shaw. How fast-folding proteins fold. *Science*, 334(6055):517–520, 2011.

Carles Domingo-Enrich, Michal Drozdzal, Brian Karrer, and Ricky T. Q. Chen. Adjoint matching: Fine-tuning flow and diffusion generative models with memoryless stochastic optimal control. *arXiv preprint arXiv:2409.08861*, 2025.

Peter Eastman, Jason Swails, John D. Chodera, Robert T. McGibbon, Yonghai Zhao, Kyle A. Beauchamp, Lee-Ping Wang, Andrew C. Simmonett, Matthew P. Harrigan, Chaya D. Stern, Rafal P. Wiewiora, Bernard R. Brooks, and Vijay S. Pande. OpenMM 7: Rapid development of high performance algorithms for molecular dynamics. *PLOS Computational Biology*, 13(7):e1005659, 2017.

Jonathan Edward King and David Ryan Koes. SidechainNet: An all-atom protein structure dataset for machine learning. *Proteins: Structure, Function, and Bioinformatics*, 89(11):1489–1496, 2021.

Christiam Camacho, George Coulouris, Vahram Avagyan, Nan Ma, Jason Papadopoulos, Kevin Bealer, and Thomas L. Madden. Blast+: Architecture and applications. *BMC Bioinformatics*, 10(421):1–9, 2009.
